# Supplementary material for: A driven quantum superconducting circuit with multiple tunable degeneracies
Source: arXiv:2211.04605 source file (2023-05-10)

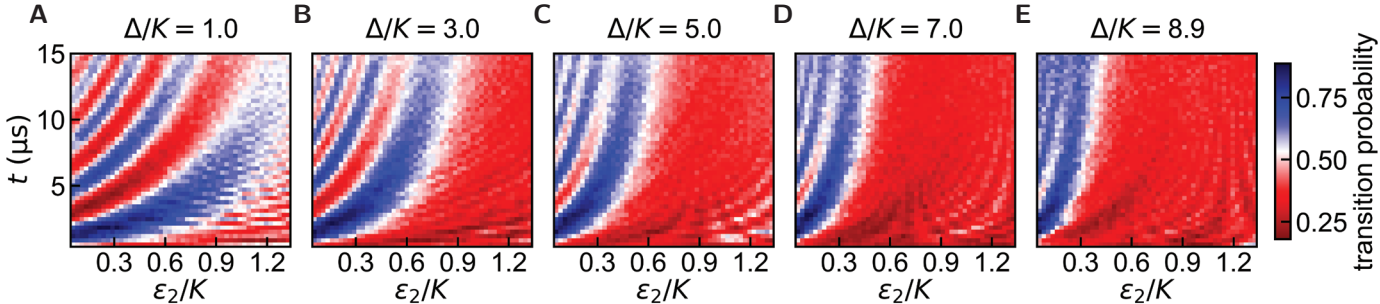

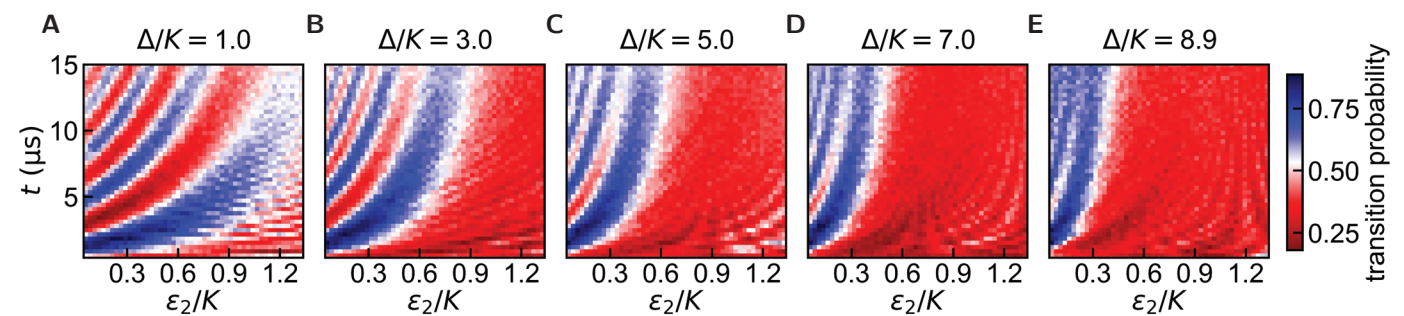

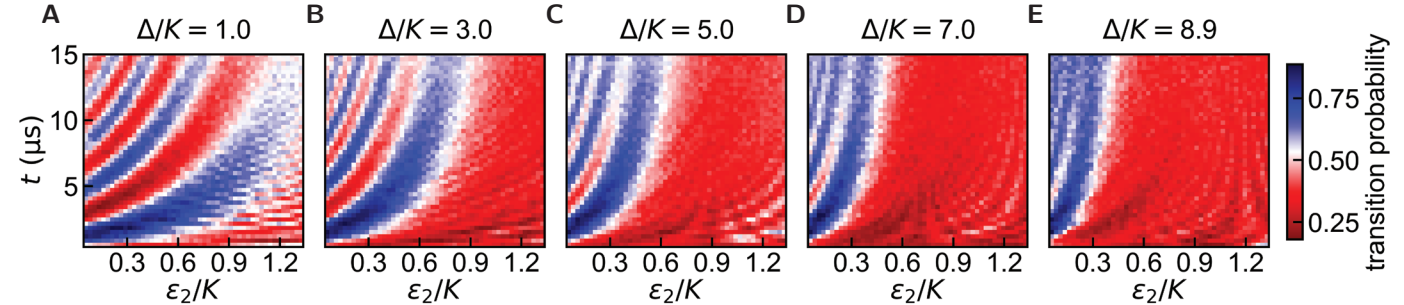

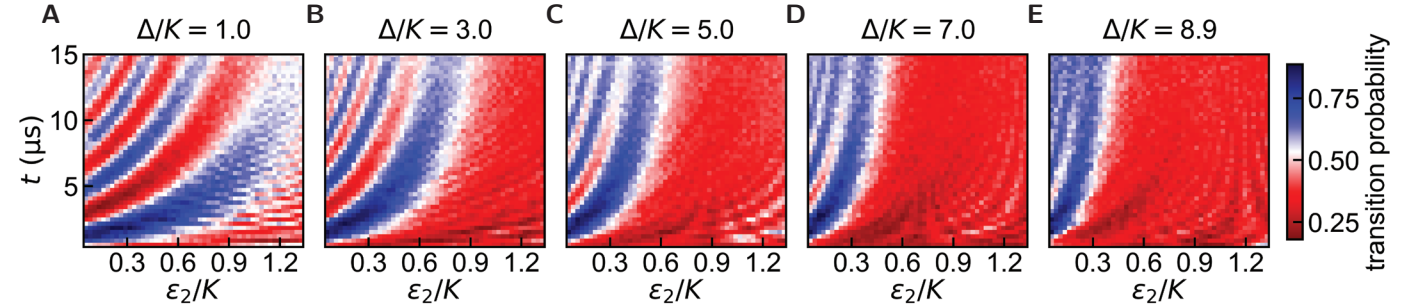

Supplement: Supplementary file 1 [file exp_supp.pdf]
